# Supplementary material for: ZKFault: Fault attack analysis on zero-knowledge based post-quantum digital signature schemes
Source: arXiv:2409.07150 source file (2024-09-11)
Supplement: Supplementary file 1 [file Lemma.tex]

\subsection{Probability of getting effective-faulted signature}\label{sec:ProbabilityEffectiveFault}

Before we start, recall that, $\vecentry{x}{2l-1},\ \vecentry{x}{2l},\ \cdots,\ \vecentry{x}{4l-2}$ are all the leaf nodes of the \textit{Reference Tree} $\vect{x}$. Let $\vecentry{x}{i}$ be the node in \textit{Reference Tree} with height $h$, and $L_{\vecentry{x}{i}}$ be the set of all leaf nodes of the subtree rooted at $\vecentry{x}{i}$. We only need the leaf nodes from $L_{\vecentry{x}{i}}$ that coincide with the first $t$ many leaf nodes of the full \textit{Reference Tree}. Let there be $v$ many such leaves, and let the set of indices of these leaves be 
$$I^{(i)}_{\text{leaf}} = \{j_1,\ j_2,\ \cdots,\ j_v\}\,.$$ 
This is the set corresponding to the node $\vecentry{x}{i}$.
%We call it as "effective leaves" of $\vecentry{x}{i}$. 
%Now, we will prove the following 
\begin{lemma}\label{lemma:effective-fault }
    If fault injection at the node $\vecentry{x}{i}$ is successful, then the probability that the fault is an "effective-fault" is 
$$\begin{cases}
1- \prod\limits_{j=0}^{v}\left(1-\frac{w}{t-j}\right) & \text{if } w>v\\
1-\prod\limits_{j=0}^{w-1}\left(\frac{v-j}{t-j}\right)-\prod\limits_{j=0}^{v}\left(1-\frac{w}{t-j}\right) & \text{otherwise}
\end{cases}$$
where $v = |I^{(i)}_{\text{leaf}}|$
%where $v$ is the number of effective leaves of $\vecentry{x}{i}$. 
\end{lemma}

\begin{proof} 
We assume the fault is successful, i.e., the instruction $Ins(i)$ has been skipped. Since all the values of the \textit{Reference Tree} $\vect{x}$ is initialized by zero, after successful-fault, the faulted \textit{Reference Tree} be $\vect{x'}$ and $\vecentry{x'}{i}=0$. Here, the following three cases may arise:\\ 
    
     \textbf{Case 1:} $\vecentry{x}{i}=0$ in non-faulted case. As we have already established, if $\vecentry{x}{i}$ is already zero, then changing its value would not mount an attack, so it is an ineffective-fault case. Now, we will find the probability of occurrence in this case, i.e., $\Pr\left[\vecentry{x}{i}=0\right]$. Now, 
    \begin{align*}
        \vecentry{x}{i}=0&\iff \text{ all the leaf nodes of the subtree rooted at }\vecentry{x}{i} \text{ are valued zero} \\
        &\iff\vecentry{x}{j}=0 ~\forall~ j\in I^{(i)}_{\text{leaf}}\iff\vecentry{f}{j-2l+1}=0 ~\forall~ j\in I^{(i)}_{\text{leaf}}\\
        &\iff\vecentry{d}{j-2l+1}=0 ~\forall~ j\in I^{(i)}_{\text{leaf}}
    \end{align*}
    Since the fixed digest vector $\vect{d}\in \ring{Z}{s}^{t}$ is an arbitrary vector of length $t$ and weight $w$, respectively, therefore the total number of all such possible vectors is $\binom{t}{w}\cdot (s-1)^w$. Also, the number of such vectors $\vect{d}$ such that the elements in the positions $\{j-2l+1:~j\in I^{(i)}_{\text{leaf}}\}$ are zero is $\binom{t-v}{w}\cdot (s-1)^w$. Therefore 
    %implies that all the  $\vecentry{d}{j-2l+1}=0$ for all $j\in I^{(i)}_{\text{leaf}}$. This case implies that all leaves of the subtree rooted at $\vecentry{x}{i}$ is zero, \textit{i.e.} $\vecentry{x}{i}=0$. As we have already established, if $\vecentry{x}{i}$ is already zero, then changing its value would not mount an attack. However, the probability that this case will occur is
    \begin{align*}
       \Pr[\vecentry{x}{i}=0]~=~ \frac{\binom{t-v}{w}\cdot (s-1)^w}{\binom{t}{w}\cdot (s-1)^w}~=~ \prod\limits_{j=0}^{v}\left(1-\frac{w}{t-j}\right) 
    \end{align*}
    \textbf{Case 2:} $\vecentry{x}{i}=1$ in the non-faulted case, and after successful fault injection $\vecentry{x'}{0}=0$. As we have already established, in this case also, we can not get information about the secret, so it is an ineffective-fault case. Now, we will find the probability of occurrence of this case, i.e., $\Pr[\vecentry{x}{i}=1 \text{ and }\vecentry{x'}{0}=0]$. 
    
    Now, $\vecentry{x}{i}=1 \text{ and }\vecentry{x'}{0}=0$ implies that all the leaf nodes with non-zero values have indices in the set $I^{(i)}_{\text{leaf}}$, otherwise $\vecentry{x'}{0}$ would have been $1$. i.e.,
    \begin{align*}
        \vecentry{x}{i}=1 \text{ and }\vecentry{x'}{0}=0&\iff \vecentry{x}{j}=0 ~\forall~ j\notin I^{(i)}_{\text{leaf}}\iff\vecentry{f}{j-2l+1}=0 ~\forall~ j\notin I^{(i)}_{\text{leaf}}\\
        &\iff\vecentry{d}{j-2l+1}=0 ~\forall~ j\notin I^{(i)}_{\text{leaf}}
    \end{align*}
    Now, $\vect{d}$ is a fixed weight vector in $\ring{Z}{s}^{t}$ with $wt(\vect{d})=w$. If $w>v$ then there must exist some $j\in I^{(i)}_{\text{leaf}}$ such that $\vecentry{d}{j-2l+1}\neq 0$. Therefore the number of vectors $\vect{d}$ such that $\vecentry{d}{j-2l+1}=0 ~\forall~ j\notin I^{(i)}_{\text{leaf}}$ is
    $$\begin{cases}
        0 & \text{if } w>v\\
        \binom{v}{w}\cdot (s-1)^w & \text{otherwise}
    \end{cases}$$
    
    %Now, the number of such vectors $\vect{d}\in \ring{Z}{s}^{t}$ such that the weight of $\vect{d}$ is $w$ and the elements in the positions $\{j-2l+1:~j\notin I_\text{leaf}\}$ are zero\\
    %= $|\{\vect{d}\in\ring{Z}{s}^{t}:~ wt(\vect{d})= w \text{ and }\vecentry{d}{j-2l+1}=0, \forall j\notin I^{(i)}_{\text{leaf}}\}|$\\
    %$
    %=|\{\vect{d_{1}}=(\vecentry{d}{j_{1}-2l+1},\ \cdots,\ \vecentry{d}{j_{v}-2l+1} )\in\ring{Z}{s}^{v}:~ wt(\vect{d_{1}})= w \}|=\begin{cases}
%0 & \text{if } w>v\\
%\binom{v}{w}\cdot (s-1)^w & \text{otherwise}
%\end{cases}$ 
Therefore,
   \begin{align*}
        \Pr[\vecentry{x}{i}=1 \text{ and }\vecentry{x'}{0}=0]
        &=\begin{cases}
0 & \text{if } w>v\\
\frac{\binom{v}{w}\cdot (s-1)^w}{\binom{t}{w}\cdot (s-1)^w} & \text{otherwise}
\end{cases}\\
&=\begin{cases}
0 & \text{if } w>v\\
\prod\limits_{i'=0}^{w-1}\left(\frac{v-i'}{t-i'}\right) & \text{otherwise}
\end{cases}  
    \end{align*}
    \textbf{Case 3:} $\vecentry{x}{i}=1$ in the non-faulted case, and after successful fault injection $\vecentry{x'}{0}=1$. As we have already established, in this case, we can get information about the secret, so it is an effective fault case. Since $\vecentry{x}{i}=1$, there exists some $j\in I^{(i)}_{\text{leaf}}$ such that $\vecentry{x}{j}=1$, i.e., $\vecentry{f}{j-2l+1}=1\implies\vecentry{d}{j-2l+1}\neq 0$. Also, since $\vecentry{x'}{0}=1$, there exists some $j'\notin I^{(i)}_{\text{leaf}}$ such that $\vecentry{x}{j'}=1$, i.e.,$\vecentry{f}{j'-2l+1}=1\implies \vecentry{d}{j'-2l+1}\neq 0$. The probability of this case occurs when neither \textbf{Case 1} nor \textbf{Case 2} occur, which is 
   $$\begin{cases}
1- \prod\limits_{i'=0}^{v}\left(1-\frac{w}{t-i'}\right) & \text{if } w>v\\
1-\prod\limits_{i'=0}^{w-1}\left(\frac{v-i'}{t-i'}\right)-\prod\limits_{i'=0}^{v}\left(1-\frac{w}{t-i'}\right) & \text{otherwise}
\end{cases}$$
This is the probability of effective fault.
\end{proof}

%  Since the products $\prod\limits_{i'=0}^{v}\left(1-\frac{w}{t-i'}\right)$ and $\prod\limits_{i'=0}^{w-1}\left(\frac{v-i'}{t-i'}\right)$  decrease in the time of $v$ increases, therefore 

%
Here, we want to get as much as possible secret information from one effective faulted signature. This will work if we can get multiple pairs $(\widetilde{\mat{Q}}_{k'},\ \mat{Q}_{\vecentry{d}{k'}}^{T}\overline{{\mat{Q}}}_{k'})$. So, we need a large number of non-zero leaf nodes of the subtree rooted at $\vecentry{x}{i}$ because then only we will get such multiple pairs from an effective faulted signature. Now, $\vecentry{x}{0}$ is the node having maximum leaf nodes, but in this case the fault will not be effective as after fault injection $\vecentry{x'}{0}$ will be zero. For this reason, we will select the node $\vecentry{x}{1}$.  %From Lemma~\ref{lemma:effective-fault }, it is evident that if $v$ increases, the probability that a successful fault is an "effective-fault" increases, where $v\geq w$. The value of $v$ depends on two things. First, the height of the node $\vecentry{x}{i}$ and second, the number of leaf nodes of the subtree rooted at $\vecentry{x}{i}$, that lies among the first $t$ many leaves of the \textit{Reference Tree} $\vect{x}$. Keeping both cases in mind, we have the maximum probability of "effective-fault" in the case where we inject fault at the node $\vecentry{x}{1}$. 
So, if the fault injection at the node $\vecentry{x}{1}$ is successful, then the probability that the fault is an "effective-fault" is $1-\prod\limits_{i'=0}^{w-1}\left(\frac{l-i'}{t-i'}\right)-\prod\limits_{i'=0}^{l}\left(1-\frac{w}{t-i'}\right)$, where $l=|I^{(1)}_{\text{leaf}}|$. Therefore the probability that the fault is an "effective-fault" is at least $\left(1-\prod\limits_{i'=0}^{w-1}\left(\frac{l-i'}{t-i'}\right)-\prod\limits_{i'=0}^{l}\left(1-\frac{w}{t-i'}\right)\right)\times p$, where $p=\Pr[\text{"successful-fault"}]$.
