# Supplementary material for: ZKFault: Fault attack analysis on zero-knowledge based post-quantum digital signature schemes
Source: arXiv:2409.07150 source file (2024-09-11)
Supplement: Supplementary file 2 [file Properties.tex]

\section{Properties of monomial matrices}\label{appendix:properties}

\noindent\textbf{Some properties:}
Let $\mat{A}=(\pi,\ \vect{u})\in M_{n}(q)$ be a invertible monomial matrix. Then, the following properties holds: %$\mat{B}=(\pi',\ \vect{u'})\in M_{n}$, $\mat{C}=(\pi_{*},\ \vect{v})\in M_{k}'$. Then the important computational actions of monomial matrices are as follows: 

\begin{enumerate}
    \item $\matentry{A}{\pi(j)}{j}=\vecentry{u}{j}$ is the only non-zero element of the $j$-th column of $\mat{A}$.\label{properties:Non-zeroElement}
    \item The transpose of the matrix $\mat{A}$ is given by 
    $$\mat{A}^{T}=(\vecentry{u}{\pi^{-1}(0)}\basisvec{\pi^{-1}(0)}~|~\cdots~|~\vecentry{u}{\pi^{-1}(n-1)}\basisvec{\pi^{-1}(n-1)})$$\label{properties:Transpose}
    \item The multiplication of any matrix $\mat{G}$ with the monomial matrix $\mat{A}$ is given by
    $$\mat{GA}=(\vecentry{u}{0}\vect{g}_{\pi(0)}~|~\cdots~|~\vecentry{u}{n-1}\vect{g}_{\pi(n-1)})$$
where $\vect{g}_{j}=\matcol{G}{j}$ is the $j$-th column of the matrix $\mat{G}$.\label{properties:Multiplication}
    \item Let $\mat{B}=(\pi', \vect{u'})\in M_n(q)$, then the multiplication of two monomial matrices $\mat{A}$ and $\mat{B}$ is given by:
    $$\mat{AB}=(\vecentry{u}{\pi'(0)}\vecentry{u'}{0}\basisvec{\pi(\pi'(0))}~|~\cdots~|~\vecentry{u}{\pi'(n-1)}\vecentry{u'}{n-1}\basisvec{\pi(\pi'(n-1))})$$\label{properties:Mono-Multiplication}
    \item The multiplication of a monomial matrices $\mat{A}$ by a partial monomial matrix $\mat{C}=(\pi_{*},\ \vect{v})\in M_{k}'(q)$ is given by:
    $$\mat{AC}=(\vecentry{u}{\pi_{*}(0)}\vecentry{v}{0}\basisvec{\pi(\pi_{*}(0))}~|~\cdots~|~\vecentry{u}{\pi_{*}(k-1)}\vecentry{v}{k-1}\basisvec{\pi(\pi_{*}(k-1))})$$\label{properties:Mono-PartialMono-Multiplication}
\end{enumerate}
\noindent\textbf{Property 1: }$\matentry{A}{\pi(j)}{j}=\vecentry{u}{j}$ is the only non-zero element of $\pi(j)$-th row as well as $j$-th column of $\mat{A}$.

Here $\mat{A}=(\vecentry{u}{0}\basisvec{\pi(0)}~|~\cdots~|~\vecentry{u}{n-1}\basisvec{\pi(n-1)})$. So, the $j$-th column of $\mat{A}$ is $\matcol{A}{j}=\vecentry{u}{j}\basisvec{\pi(j)}$. Since $\basisvec{\pi(j)}$ is a basis vector, all the elements of $\matcol{A}{j}$ are zero except the $\pi(j)$-th element, which is $\vecentry{u}{j}$. So, for each $j$-th column, $\matentry{A}{\pi(j)}{j}=\vecentry{u}{j}$ is the only non-zero element. Also, since $\pi$ is a permutation, the position of the non-zero element of each column is distinct, i.e., $\matentry{A}{\pi(j)}{j}$ is the only non-zero element in $\pi(j)$-th row of the matrix $\mat{A}.$ Hence, for each $j$, $\matentry{A}{\pi(j)}{j}=\vecentry{u}{j}$ is the only non-zero element of $\pi(j)$-th row as well as $j$-th column of $\mat{A}$.\\

\noindent\textbf{Property 2: }The transpose of the matrix $\mat{A}$ is given by 
    $$\mat{A}^{T}=(\vecentry{u}{\pi^{-1}(0)}\basisvec{\pi^{-1}(0)}~|~\cdots~|~\vecentry{u}{\pi^{-1}(n-1)}\basisvec{\pi^{-1}(n-1)})$$

Enough to show that the $j$-th column of $\mat{A}^{T}$ is $\vecentry{u}{\pi^{-1}(j)}\basisvec{\pi^{-1}(j)}$. Now, the $j$-th column of $\mat{A}^{T}$ = $j$-th row of $\mat{A}$. From the property 1, we know that $\matentry{A}{j}{\pi^{-1}(j)}=\vecentry{u}{\pi^{-1}(j)}$ is the only non-zero element in the $j$-th row as well as $\pi^{-1}(j)$-th column of $\mat{A}$ i.e., the $j$-th row of $\mat{A}$ is, $\matrow{A}{j}=\vecentry{u}{\pi^{-1}(j)}\basisvec{\pi^{-1}(j)}$. Therefore, the $j$-th column of $\mat{A}^{T}=\vecentry{u}{\pi^{-1}(j)}\basisvec{\pi^{-1}(j)}$.\\

\noindent\textbf{Property 3: } The multiplication of any matrix $\mat{G}=(\vect{g}_{0}~|~\cdots~|~\vect{g}_{n-1})$, by the monomial matrix $\mat{A}$ is given by
    $$\mat{GA}=(\vecentry{u}{0}\vect{g}_{\pi(0)}~|~\cdots~|~\vecentry{u}{n-1}\vect{g}_{\pi(n-1)})$$
where $\vect{g}_{j}=\matcol{G}{j}$ is the $j$-th column of the matrix $\mat{G}$.\\

Enough to show that the $j$-th column of $\mat{GA}$ is $\vecentry{u}{j}\vect{g}_{\pi(j)}$. Now, the $i,\ j$-th element of $\mat{GA}$ is given by:
$$\matentry{GA}{i}{j}=\sum_{k=0}^{n-1}\matentry{G}{i}{k}\matentry{A}{k}{j}=\matentry{G}{i}{\pi(j)}\matentry{A}{\pi(j)}{j},$$
since $\matentry{A}{\pi(j)}{j}$ is the only non-zero element in the $j$-th column of $\mat{A}$. 
Therefore the $j$-th column of $\mat{GA}$ is given by
$$\matcol{GA}{j}=\matcol{G}{\pi(j)}\matentry{A}{\pi(j)}{j}=\vect{g}_{\pi(j)}\vecentry{u}{j}=\vecentry{u}{j}\vect{g}_{\pi(j)}$$\\

\noindent\textbf{Property 4: }The multiplication of two monomial matrices $\mat{A}$ and $\mat{B}=(\pi',\ \vect{u'})\in M_{n}$ is given by:
    $$\mat{AB}=(\vecentry{u}{\pi'(0)}\vecentry{u'}{0}\basisvec{\pi(\pi'(0))}~|~\cdots~|~\vecentry{u}{\pi'(n-1)}\vecentry{u'}{n-1}\basisvec{\pi(\pi'(n-1))})$$
    
Enough to show that the $j$-th column of $\mat{AB}$ is $\vecentry{u}{\pi'(j)}\vecentry{u'}{j}\basisvec{\pi(\pi'(j))}$. From the property 3, we have the $j$-th column of $\mat{AB}$ is given by:
$$\matcol{AB}{j}=\vecentry{u'}{j}\matcol{A}{\pi'(j)}$$
Since the $j$-th column of $\mat{A}$ is $\matcol{A}{j}=\vecentry{u}{j}\basisvec{\pi(j)}$, therefore the $\pi'(j)$-th column of $\mat{A}$ will be $\matcol{A}{\pi'(j)}=\vecentry{u}{\pi'(j)}\basisvec{\pi(\pi'(j))}$. Hence, the $j$-th column of $\mat{AB}$ will be 
$\vecentry{u}{\pi'(j)}\vecentry{u'}{j}\basisvec{\pi(\pi'(j))}$.\\

\noindent\textbf{Property 5: } The multiplication of a monomial matrices $\mat{A}$ by a partial monomial matrix $\mat{C}=(\pi_{*},\ \vect{v})\in M_{k}'$ is given by:
    $$\mat{AC}=(\vecentry{u}{\pi_{*}(0)}\vecentry{v}{0}\basisvec{\pi(\pi_{*}(0))}~|~\cdots~|~\vecentry{u}{\pi_{*}(k-1)}\vecentry{v}{k-1}\basisvec{\pi(\pi_{*}(k-1))})$$

Similar to property 4.
\iffalse
Let $\mat{G}=(\vect{g}_{0}~|~\vect{g}_{1}~|~\cdots~|\vect{g}_{n-1})$ be a matrix of order $k\times n$ and $\mat{A}=(\pi,\ \vect{u})\in M_{n}$. Then, the following properties holds: %$\mat{B}=(\pi',\ \vect{u'})\in M_{n}$, $\mat{C}=(\pi_{*},\ \vect{v})\in M_{k}'$. Then the important computational actions of monomial matrices are as follows: 

\begin{enumerate}
    \item $\matentry{A}{\pi(j)}{j}=\vecentry{u}{j}$ is the only non-zero element of $\pi(j)$-th row as well as $j$-th column of $\mat{A}$.\label{properties:Non-zeroElement}
    \item The transpose of the matrix $\mat{A}$ is given by 
    $$\mat{A}^{T}=(\vecentry{u}{\pi^{-1}(0)}\basisvec{\pi^{-1}(0)}~|~\cdots~|~\vecentry{u}{\pi^{-1}(n-1)}\basisvec{\pi^{-1}(n-1)})$$\label{properties:Transpose}
    \item The matrix $\mat{GA}$ is given by
    $$\mat{GA}=(\vecentry{u}{\pi(0)}\vect{g}_{\pi(0)}~|~\cdots~|~\vecentry{u}{\pi(n-1)}\vect{g}_{\pi(n-1)})$$\label{properties:Multiplication}
    \item The multiplication of two monomial matrices $\mat{A}$ and $\mat{B}=(\pi',\ \vect{u'})\in M_{n}$ is given by:
    $$\mat{AB}=(\vecentry{u}{\pi'(0)}\vecentry{u'}{0}\basisvec{\pi(\pi'(0))}~|~\cdots~|~\vecentry{u}{\pi'(n-1)}\vecentry{u'}{n-1}\basisvec{\pi(\pi'(n-1))})$$\label{properties:Mono-Multiplication}
    \item The multiplication of a monomial matrices $\mat{A}$ by a partial monomial matrix $\mat{C}=(\pi_{*},\ \vect{v})\in M_{k}'$ is given by:
    $$\mat{AC}=(\vecentry{u}{\pi_{*}(0)}\vecentry{v}{0}\basisvec{\pi(\pi_{*}(0))}~|~\cdots~|~\vecentry{u}{\pi_{*}(k-1)}\vecentry{v}{k-1}\basisvec{\pi(\pi_{*}(k-1))})$$\label{properties:Mono-PartialMono-Multiplication}
\end{enumerate}
\fi
