# Supplementary material for: ZKFault: Fault attack analysis on zero-knowledge based post-quantum digital signature schemes
Source: arXiv:2409.07150 source file (2024-09-11)
Supplement: Supplementary file 3 [file Protocols.tex]

\section{Some interacting protocols}\label{appendix:protocols}
Here the parameters $q,\ n,\ k \in \mathbb{N}$, matrix $\mat{G}_{0} \in \fieldmat{F}{q}{k}{n}$ and
a hash function $\texttt{H}$ are public. The private key for the prover is a monomial matrix $\mat{Q}\in M_{n}$ and the public key is $\mat{G}_{1}=\texttt{RREF}(\mat{G}_{0}\mat{Q}^{-T})$. The interaction between the prover and the verifier is described in the protocol in Fig.~\ref{fig:Sigma_protocol}. 

\begin{figure}[!ht]
%\centering
\includegraphics[width=1\linewidth]{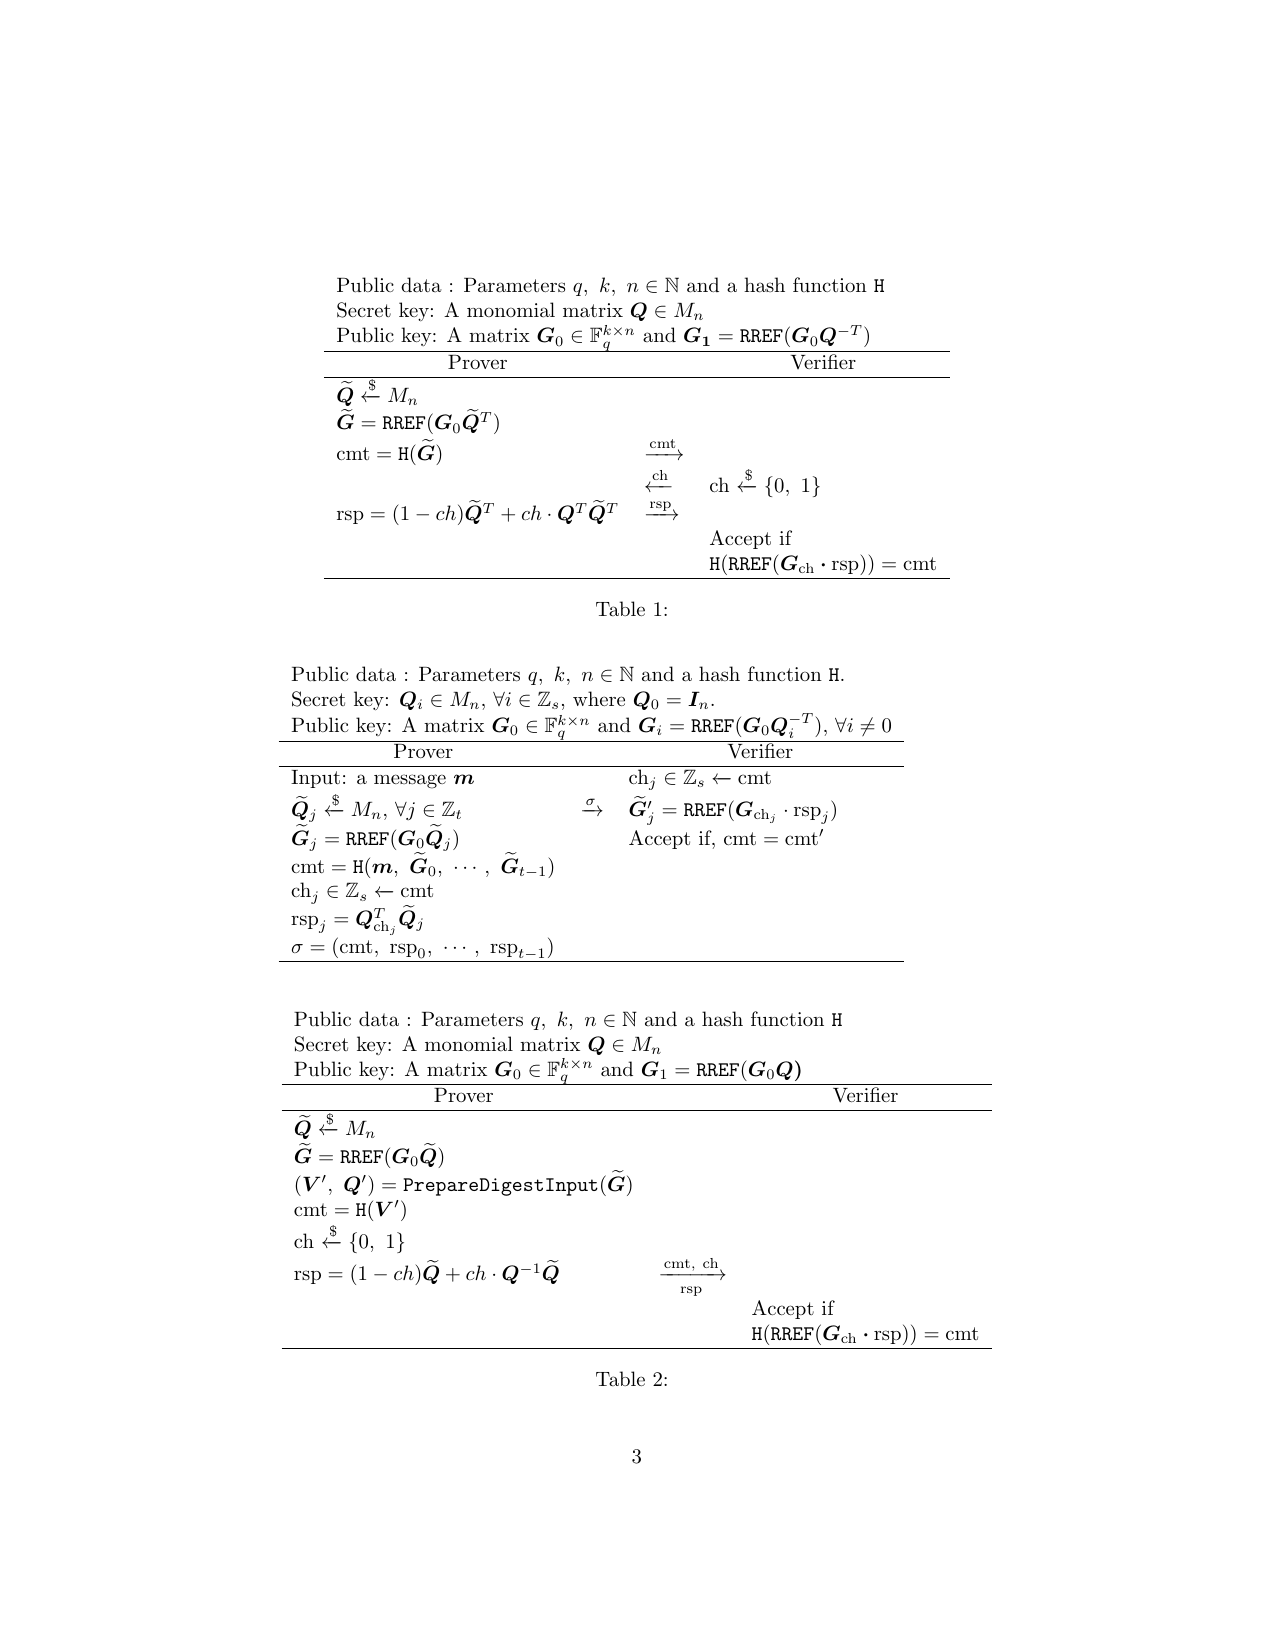}
\caption{LESS-v1 identification scheme~\cite{LESS_is_More}. }
\label{fig:Sigma_protocol}  
\end{figure}

\noindent\textbf{Completeness: } To check the completeness of the protocol, it is to show that for a valid $(\text{cmt,\ ch,\ rsp})$ is always accepted $i.e.$, $\texttt{H}(\texttt{RREF}(\mat{G}_{\text{ch}}\cdot \text{rsp}))$ will be equal to $\text{cmt}$. If \texttt{H} is a collision-resistant hash function, then it is enough to show that for any $\text{ch}\in \left\{0,\ 1\right\}$, $\texttt{RREF}(\mat{G}_{\text{ch}}\cdot \text{rsp})=\widetilde{\mat{G}}$.
\begin{itemize}
    \item \textbf{Case 1: }For $\text{ch}=0$, $\text{rsp}=\widetilde{\mat{Q}}^{T}$. In this case, $\texttt{RREF}(\mat{G}_{\text{ch}}\cdot \text{rsp}))=\texttt{RREF}(\mat{G}_{0}\cdot \widetilde{\mat{Q}}^{T}) = \widetilde{\mat{G}}.$
    
    \item \textbf{Case 2: }For $\text{ch}=1$, $\text{rsp}=\mat{Q}^{T}\widetilde{\mat{Q}}^{T}$, so in this case, $\texttt{RREF}(\mat{G}_{\text{ch}}\cdot \text{rsp}))=\texttt{RREF}(\mat{G}_{1}\cdot \mat{Q}^{T}\widetilde{\mat{Q}}^{T}).$ Since $\mat{G}_{1}=\texttt{RREF}(\mat{G}_{0}\mat{Q}^{-T})$, there exists a non-singular matrix $\mat{E}$ such that $\mat{G}_{1}=\mat{EG}_{0}\mat{Q}^{-T}$. Hence, $$\texttt{RREF}(\mat{G}_{1}\cdot \mat{Q}^{T}\widetilde{\mat{Q}}^{T})=\texttt{RREF}(\mat{EG}_{0}\mat{Q}^{-T}\cdot\mat{Q}^{T} \widetilde{\mat{Q}}^{T})=\texttt{RREF}(\mat{EG}_{0}\widetilde{\mat{Q}}^{T})$$
     Also, since $\widetilde{\mat{G}}=\texttt{RREF}(\mat{G}_{0}\widetilde{\mat{Q}}^{T})$, there exists a non-singular matrix $\mat{E}'$ such that $\widetilde{\mat{G}}=\mat{E}'\mat{G}_{0}\widetilde{\mat{Q}}^{T}$. We can write $\widetilde{\mat{G}}$ as $$\widetilde{\mat{G}}=\mat{E}'\mat{G}_{0}\widetilde{\mat{Q}}^{T}=\mat{E}'\mat{E}^{-1}(\mat{E}\mat{G}_{0}\widetilde{\mat{Q}}^{T})$$ Since $\widetilde{\mat{G}}$ is in $\texttt{RREF}$ and the $\texttt{RREF}$ of a matrix is unique, therefore $\texttt{RREF}(\mat{EG}_{0}\widetilde{\mat{Q}}^{T})=\widetilde{\mat{G}}$.
     So, for $\text{ch}=1$, $\texttt{RREF}(\mat{G}_{\text{ch}}\cdot \text{rsp})=\texttt{RREF}(\mat{EG}_{0}\widetilde{\mat{Q}}^{T})=\widetilde{\mat{G}}$. 
\end{itemize}
Therefore, for any $\text{ch}\in \left\{0,\ 1\right\}$, $\texttt{RREF}(\mat{G}_{\text{ch}}\cdot \text{rsp})=\widetilde{\mat{G}}$, hence, proves that protocol is correct. Also in the protocol in Fig.~\ref{fig:Sigma_protocol}, an honest verifier achieves no information about the secret. This assertion follows from the next Lemma.

\begin{lemma}
For any $\mat{Q}\in M_{n}$ and $\widetilde{\mat{Q}}\xleftarrow[]{\$}M_{n}$, the multiplication matrix $\mat{Q}^{T}\widetilde{\mat{Q}}^{T}$ follows a uniform distribution over the set $M_{n}$~\cite{LESS_is_More}. 
\end{lemma}
When $\text{ch} = 0$, the verifier receives $\text{rsp}=\widetilde{\mat{Q}}^{T}$ as a response, which does not reveal any information about the secret matrix $\mat{Q}$. Similarly, when $\text{ch} = 1$, the verifier gets $\mat{Q}^{T}\widetilde{\mat{Q}}^{T}$ as a response, and since this matrix is uniformly distributed over $M_{n}$, the verifier gains no information about $\mat{Q}$. This holds in either case, ensuring that the verifier remains completely unaware of the secret matrix $\mat{Q}$.\\

\noindent\textbf{Soundness: }The protocol in Fig. ~\ref{fig:Sigma_protocol} is 2-special sound $i.e.$ if we are given two valid transcripts $\text{tr}_{0}=(\text{cmt},\ \text{ch}=0,\ \text{rsp}= \widetilde{\mat{Q}}^{T})$ and $\text{tr}_{1}=(\text{cmt},\ \text{ch}=1,\ \text{rsp}=\mat{Q}^{T}\widetilde{\mat{Q}}^{T})$, then we can find the witness $\mat{Q}$. Next, we calculate the soundness error of this protocol. Let the dishonest prover Eve makes two transcripts as $\text{tr}_{0}=(\text{cmt},\ \text{ch}=0,\ \text{rsp}= \widetilde{\mat{Q}}^{T})$ and $\text{tr}_{1}=(\text{cmt},\ \text{ch}=1,\ \text{rsp}={\mat{Q}}^{*})$, where $\text{cmt}=\texttt{H}(\texttt{RREF}(\mat{G}_{0}\widetilde{\mat{Q}}^{T}))$ and $\mat{Q}^{*}\xleftarrow[]{\$}M_{n}$. Then 
\begin{align*}
    &Pr[\text{Eve will win}]\\
    &=Pr[\text{ch}=0]\cdot Pr[\text{tr}_{0} \text{ is satisfied}~|~\text{ch}=0]+Pr[\text{ch}=1]\cdot Pr[\text{tr}_{1} \text{ is satisfied}~|~\text{ch}=1]\\
    &=\frac{1}{2} (Pr[\text{tr}_{0} \text{ is satisfied}~|~\text{ch}=0]+ Pr[\text{tr}_{1} \text{ is satisfied}~|~\text{ch}=1])
\end{align*}
Now, for the first transcript $\text{tr}_{0}$, $\texttt{H}(\texttt{RREF}(\mat{G}_{\text{ch}}\cdot \text{rsp}))=\texttt{H}(\texttt{RREF}(\mat{G}_{0}\cdot \widetilde{\mat{Q}}^{T}))=\text{cmt}.$ So if $\text{ch}=0$, then the transcript $\text{tr}_{0}$ will always satisfies. Hence, $Pr[\text{tr}_{0} \text{ is satisfied}~|~\text{ch}=0]=1.$ But, if $\text{ch}=1$, then the transcript $\text{tr}_{1}$ will be satisfied if Eve selects the matrix $\mat{Q}^{*}$ as response such that $\texttt{H}(\texttt{RREF}(\mat{G}_{1}\mat{Q}^{*}))=\text{cmt}=\texttt{H}(\texttt{RREF}(\mat{G}_{0} \widetilde{\mat{Q}}^{T})).$ Since $\texttt{H}$ is collision resistant hash function, therefore
\begin{align*}
   \texttt{RREF}(\mat{G}_{1}\mat{Q}^{*})&=\texttt{RREF}(\mat{G}_{0}\widetilde{\mat{Q}}^{T})\\
   \implies \mat{G}_{1} \mat{Q}^{*}&=\mat{SG}_{0} \widetilde{\mat{Q}}^{T}, \text{ for some }\mat{S}\in \text{GL}_{k}\implies \mat{G}_{1}=\mat{SG}_{0} \widetilde{\mat{Q}}^{T}\mat{Q}^{*-1}
\end{align*}
   So, here the prover has to find the monomial matrix $\mat{Q}^{*}$ and a non-singular matrix $S$ such that the previous equation $\mat{G}_{1}=\mat{SG}_{0} \widetilde{\mat{Q}}^{T}\mat{Q}^{*-1}$ holds, and this is the computational version of linear code equivalence problem, which assume to be hard. Therefore, $Pr[\text{tr}_{1} \text{ is satisfied}~|~\text{ch}=1]=\epsilon$, where $\epsilon<<1$. Hence, $
    Pr[\text{Eve will win}]\sim \frac{1}{2}$. \\
    
One can observe that for a dishonest prover, the verifier accepts the response with probability atleast $\frac{1}{2}$. This implies that the soundness error of this identification protocol is atleast $\frac{1}{2}$. However, this protocol can be repeated multiple times to reduce this soundness error. The protocol in Fig.~\ref{fig:Canonical_Identification} reduces the soundness error from $\frac{1}{2}$ to $\frac{1}{2^{st}}$, where $s-1$ is the number of secret monomial matrices and $t$ is the size of the $\text{ch}$ array. This is the modified version of the protocol in Fig.~\ref{fig:Sigma_protocol}.

\begin{figure}[h]
%\centering
\includegraphics[width=1\linewidth]{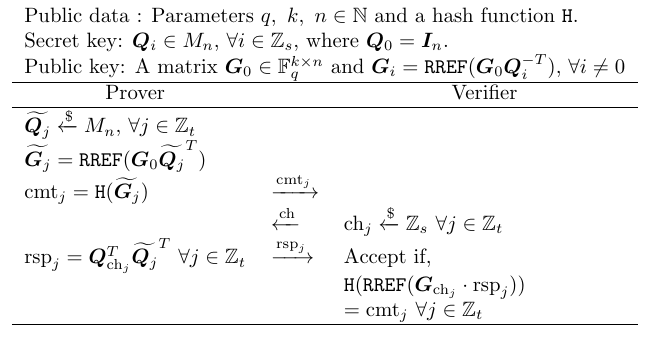}
\caption{The canonical LESS-v1 identification scheme~\cite{LESS_is_More}. }
\label{fig:Canonical_Identification}  
\end{figure}
\begin{figure}[h]
%\centering
\includegraphics[width=1\linewidth]{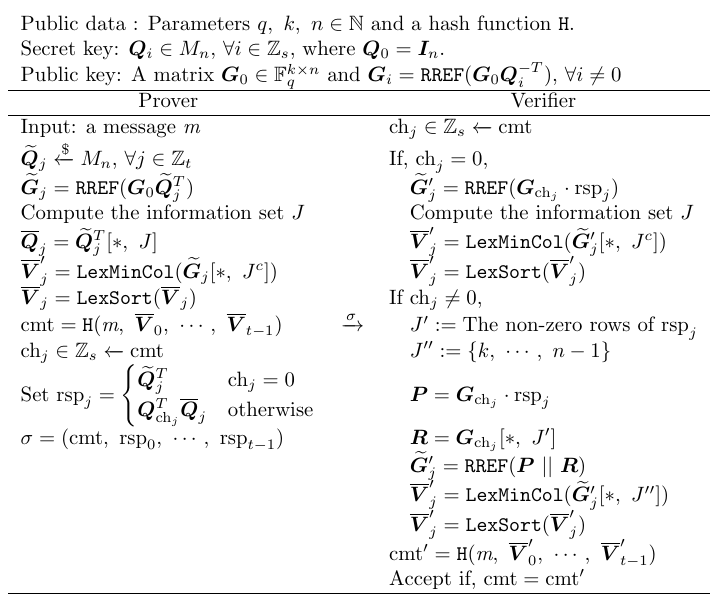}
\caption{Final version of LESS. }
\label{fig:Less_final}  
\end{figure}
\begin{lemma}\label{lemma:Less_final}
    The response from an honest prover in the protocol in Fig.~\ref{fig:Less_final}, is always accepted by the verifier.  
\end{lemma}

\begin{proof}
If $\text{ch}_{j}=0$, then clearly $\overline{\mat{V}}_{j}=\overline{\mat{V}}_{j}'$ holds. Now, our goal is to demonstrate that for $\text{ch}_{j}\neq 0$, $\overline{\mat{V}}_{j}=\overline{\mat{V}}_{j}'$ holds.
Let $\mat{Q}_{\text{ch}_{j}}^{T}=(\pi,\ \vect{v})$ and $\widetilde{\mat{Q}}_{j}^{T}=(\pi',\ \vect{v}')$ be two monomial matrices. Consider $\mat{G}_{0}=(\vect{g}_{0}|\vect{g}_{1}|\cdots|\vect{g}_{n-1})$ as the generator matrix where each $\vect{g}_{i}=\mat{G}_{0}[*, i]$ is the $i$-th column of the matrix $\mat{G}_{0}$. Define $\mat{G}_{\text{ch}_{j}}=\texttt{RREF}(\mat{G}_{0}\mat{Q}_{\text{ch}_{j}}^{-T})$ and $\widetilde{\mat{G}}_{j}=\texttt{RREF}(\mat{G}_{0}\widetilde{\mat{Q}}_{j}^{T})$.
Let $\mat{G}=\mat{G}_{0}\widetilde{\mat{Q}}_{j}^{T}$ and $J$ be the information set of the code $\mat{G}$. Then, $\widetilde{\mat{G}}_{j}=\matcol{G}{J}^{-1}\mat{G}=\matcol{G}{J}^{-1}\mat{G}_{0}\widetilde{\mat{Q}}_{j}^{T}$ holds. This implies, \begin{align*}
   & \widetilde{\mat{G}}_{j}[*,\ J^{c}]=\matcol{G}{J}^{-1}\mat{G}_{0}\widetilde{\mat{Q}}_{j}^{T}[*,\ J^{c}]
\end{align*}
Now the $i$-column of the matrix $\mat{G}_{0}\widetilde{\mat{Q}}_{j}^{T}[*,\ J^{c}]$ is given by $\vecentry{v'}{j_{i}}\vect{g}_{\pi'(j_{i})}$, where $j_{i}$ is the $i$-th element of the ordered set $J^{c}$.
Therefore, the matrix $\widetilde{\mat{G}}_{j}[*,\ J^{c}]$ will be $\widetilde{\mat{G}}_{j}[*,\ J^{c}]=(\vecentry{v'}{j_{0}}\matcol{G}{J}^{-1}\vect{g}_{\pi'(j_{0})}~|~\cdots~|~\vecentry{v'}{j_{k-1}}\matcol{G}{J}^{-1}\vect{g}_{\pi'(j_{k-1})})$, for all $j_{i}\in J^{c}$.
Considering that $\vecentry{v'}{j_{i}}$ is a non-zero scalar, for all $j_{i}\in J^{c}$, we have:
\begin{align*}
        &\texttt{LexMinCol}(\vecentry{v'}{j_{i}}\matcol{G}{J}^{-1}\vect{g}_{\pi'(j_{i})})
        =\texttt{LexMinCol}(\matcol{G}{J}^{-1}\vect{g}_{\pi'(j_{i})})\\
    \implies &\texttt{LexMinCol}(\widetilde{\mat{G}}_{j}[*,\ J^{c}])
        =\texttt{LexMinCol}(\mat{B})
\end{align*}
where $\matcol{G}{J}^{-1}\vect{g}_{\pi'(j_{i})}$ is the $i$-th column of the matrix $\mat{B}$. Therefore, $$\overline{\mat{V}}_{j}=\texttt{LexSort}(\texttt{LexMinCol}(\widetilde{\mat{G}}_{j}[*,\ J^{c}]))=\texttt{LexSort}(\texttt{LexMinCol}(B))$$
To prove $\overline{\mat{V}}_{j}=\overline{\mat{V}}_{j}'$, it suffices to demonstrate that each column of $\widetilde{\mat{G}}_{j}'[*, J'']$ is a non-zero scaler multiple of some column of $\mat{B}$. Considering the relationship $\mat{Q}_{\text{ch}_{j}}^{T}\overline{\mat{Q}}_{j}=\mat{Q}_{\text{ch}_{j}}^{T}\widetilde{\mat{Q}}_{j}^{T}[*,\ J]$, we obtain $J'=\ring{Z}{n}\setminus\left\{\pi(\pi'(j)): j\in J\right\}=\left\{\pi(\pi'(j)): j\in J^{c}\right\}$, representing the positions of zero rows in the matrix $\mat{Q}_{\text{ch}_{j}}^{T}\overline{\mat{Q}}_{j}$.
Now, $\mat{P}=\mat{G}_{\text{ch}_{j}}\cdot \text{rsp}_{j}=\mat{G}_{\text{ch}_{j}}\cdot \mat{Q}_{\text{ch}_{j}}^{T}\overline{\mat{Q}}_{j}$ and $\mat{R}=\mat{G}_{\text{ch}_{j}}[*, J']$. Since $\mat{G}_{\text{ch}_{j}}=\texttt{RREF}(\mat{G}_{0}\mat{Q}_{\text{ch}_{j}}^{-T})$, therefore there exists a matrix $\mat{S}\in GL_{k}(q)$ such that $\mat{G}_{\text{ch}_{j}}=\mat{SG}_{0}\mat{Q}_{\text{ch}_{j}}^{-T}$. Therefore,
\begin{align*}
&\mat{P}=\mat{S}\mat{G}_{0}\mat{Q}_{\text{ch}_{j}}^{-T}\cdot \mat{Q}_{\text{ch}_{j}}^{T}\overline{\mat{Q}}_{j}=\mat{S}\mat{G}_{0}\overline{\mat{Q}}_{j} \text{ and }
\mat{R}=\mat{S}\mat{G}_{0}\mat{Q}_{\text{ch}_{j}}^{-T}[*,\ J']
\end{align*}
Now,
\begin{align*}
\widetilde{\mat{G}}_{j}'&=\texttt{RREF}\left(\mat{P}~|~\mat{R}\right)=\texttt{RREF}(\mat{S}\mat{G}_{0}\overline{\mat{Q}}_{j}~|~\mat{S}\mat{G}_{0}\mat{Q}_{\text{ch}_{j}}^{-T}[*,\ J'])=\texttt{RREF}(\mat{G}_{0}\overline{\mat{Q}}_{j}~|~\mat{G}_{0}\mat{Q}_{\text{ch}_{j}}^{-T}[*,\ J'])\\
&=\texttt{RREF}(\matcol{G}{J}~|~\mat{G}_{0}\mat{Q}_{\text{ch}_{j}}^{-T}[*,\ J'])=(\mathbf{I}_{k}~|~\matcol{G}{J}^{-1}\mat{G}_{0}\mat{Q}_{\text{ch}_{j}}^{-T}[*,\ J']),
\end{align*}
since $J$ is the information set of $\mat{G}$. Therefore 
$\widetilde{\mat{G}}_{j}'[*,\ J'']=\matcol{G}{J}^{-1}\mat{G}_{0}\mat{Q}_{\text{ch}_{j}}^{-T}[*,\ J']$. Therefore, each column of $\widetilde{\mat{G}}_{j}'[*,\ J'']$ is a multiple of the term $\matcol{G}{J}^{-1}\vect{g}_{\pi^{-1}(j')}$, where $j'\in J'$. Since $J'=\left\{\pi(\pi'(j')):j'\in J^{c}\right\}$, each column of $\widetilde{\mat{G}}_{j}'[*,\ J'']$ is a multiple of $\matcol{G}{J}^{-1}\vect{g}_{\pi'(j_{i})}$, where $j_{i}\in J^{c}$. Thus, $\overline{\mat{V}}_{j}'=\texttt{LexSort}(\mat{B})=\overline{\mat{V}}_{j}$.
The completeness of the protocol illustrated in Fig.~\ref{fig:Less_final} is established.

\end{proof}
